# Supplementary material for: This is SpArta: Rigorous Optimization of Regionally Resolved Energy Systems by Spatial Aggregation and Decomposition
Source: arXiv:2302.05222 source file (2023-02-10)
Supplement: Supplementary file 1 [file appendix.tex]

\appendix
\label{Appendix}
\section{Risk-neutral asset-backed trading strategy}
\label{sec:abt_strategy}

Fig.~\ref{fig:abt_strategy} exemplifies the risk-neutral asset-backed trading strategy in the multiperiod binomial model for positive flexible capacity.
%In Fig.~\ref{fig:abt_strategy}, we consider positive flexible capacity.
For negative flexible capacity, the multiperiod binomial model works similarly but in the opposite direction.

The relative electricity output $y$ is the relative flexible capacity traded on the continuous intraday market.
At each trading opportunity, the trader adjusts the sold share of flexible capacity $y$.
The adjustment is based on the stochastic price process, and the marginal electricity costs $mc$.
%is potentially delivered to the market depending on the trades in the continuous intraday market.
Therein, the trader behaves risk-neutral to realize the estimated option value $opt$ within the trading session.
The option value is realized independent of the price scenario I, II, and III.
At the end of a trading session, the price volatility in the continuous intraday market is monetized to the option value.
The positive flexible capacity is either entirely sold ($y=1$) or not ($y=0$).

For further information regarding the explicit computation of the risk-neutral asset-backed trading strategy, we refer to \citet{Bjork.2009}.

\begin{figure}[h!]
    \centering
	\includegraphics[width=9cm]{Figures/asset_backed_trading_small_new.pdf}
 	\caption{Exemplary risk-neutral asset-backed trading strategy for positive flexible capacity in the multiperiod binomial model based on \citep{Cox.1979}. Each discrete price offers a trading opportunity at which the trader adjusts the share of sold flexible capacity $y$ to realize the option value $opt$ independent of scenarios I, II, and III.}
	\label{fig:abt_strategy}
\end{figure}

%%%%%%%%%%%%%%%%%%%%%%%%%%%%%%%%%%%%%%%%%%%%%%%%%%%
%\textbf{Risk-neutral asset-backed trading strategy}
%%%%%%%%%%%%%%%%%%%%%%%%%%%%%%%%%%%%%%%%%%%%%%%%%%%
%At the end of a trading session, the option value is realized independent of scenario I, II, and III. However, depending on the stochastic price process compared to the marginal electricity costs, the flexible capacity is either entirely sold ($y=1$ if last price $>$ marginal electricity costs $mc$) or not ($y=0$ if last price $<$ marginal electricity costs $mc$).
 	 % Exemplary, $opt^I$ is calculated as the difference of the trading position multiplied with the current electricity price substracted by the marginal electricity costs as electricity is delivered in scenario I.}

\clearpage

\section{Installed units of the multi-energy system}

\begin{table}[!h]
	\caption[Units of the decentralized energy system]{Overview of the installed units of the multi-energy system, their electrical and thermal capacities, and their output. AC: absorption chillers, CC: compression chillers, B: boilers, EB: electrode boilers, and CHP: combined heat and power units.}
	\vspace{6pt}
	\centering	
	\begin{tabular}{llll} 
	\toprule
	\textbf{Component}	&	\textbf{Capacity} [\si{\mega\watt}\textsubscript{el}] &	\textbf{Capacity} [\si{\mega\watt}\textsubscript{th}]	&	\textbf{Output}\\
	\midrule 
	AC 1 		& &	3.5	&	Cooling\\
	AC 2		& &	2.5 	&		\\
	AC 3		& &	0.5 	&		\\
	\midrule 
	CC 1		& 0.8 &	4.5 	&	Cooling\\
	CC 2		& 0.4 &	2.5 	&		\\
	CC 3		& 0.1 &	0.5 	&		\\
	\midrule
	B 1		& &	4.0 &	Heating\\
	B 2		& &	3.0 &		\\
	B 3		& &	3.0 &		\\
	B 4 	& &	1.0	&		\\	
	\midrule
	EB 1	& 1.5 &	1.5 	&	Heating\\	
	EB 2	& 1.0 &	1.0		&		\\
	\midrule
	CHP 1	& 4.4 & 4	&	Heating, Electricity	\\
	CHP 2	& 2.2 &	2   &	 \\
	CHP 3	& 2.2 &	2   &	 \\
	CHP 4	& 1.1 &	1  	&		\\
	\bottomrule 
	\end{tabular}
\label{tab:components}
\end{table}

\clearpage
%\FloatBarrier
